# Supplementary material for: Viscotaxis of chiral microswimmer in viscosity gradients
Source: arXiv:2501.02805 ancillary file (2025-01-06)
Supplement: Supplementary file 1 [file SM.pdf]

# Viscotaxis of chiral microswimmer in viscosity gradients—supplemental material

Takuya Kobayashi[1] and Ryoichi Yamamoto[1]
[1]Department of Chemical Engineering, Kyoto University, Kyoto 615-8510, Japan
(Dated: January 4, 2025)

## S1. INTEGRAL THEOREM FOR FLUIDS WITH VISCOSITY GRADIENTS

We consider an incompressible fluid flow in the Stokes limit,

$$\boldsymbol{\nabla} \cdot \boldsymbol{u} = 0, \qquad \boldsymbol{\nabla} \cdot \boldsymbol{\sigma} = \boldsymbol{0}, \tag{S1}$$

where $\boldsymbol{u}$ and $\boldsymbol{\sigma}$ represent the velocity and stress fields, respectively.

We revisit the integral theorem to derive the swimming speed of a chiral squirmer in viscosity gradients without needing to calculate the flow fields directly [S1, S2]. We choose $\hat{\boldsymbol{u}}$ and $\hat{\boldsymbol{\sigma}}$, governed by the Stokes equation with constant viscosity $\eta_0$, as an auxiliary problem, and start with the identities,

$$\boldsymbol{\nabla} \cdot (\boldsymbol{\sigma} \cdot \hat{\boldsymbol{u}}) = (\boldsymbol{\nabla} \cdot \boldsymbol{\sigma}) \cdot \hat{\boldsymbol{u}} + \boldsymbol{\sigma} : \boldsymbol{\nabla}\hat{\boldsymbol{u}}, \tag{S2a}$$
$$\boldsymbol{\nabla} \cdot (\hat{\boldsymbol{\sigma}} \cdot \boldsymbol{u}) = (\boldsymbol{\nabla} \cdot \hat{\boldsymbol{\sigma}}) \cdot \boldsymbol{u} + \hat{\boldsymbol{\sigma}} : \boldsymbol{\nabla}\boldsymbol{u}, \tag{S2b}$$

where $\boldsymbol{A} : \boldsymbol{B} = A_{ij}B_{ij}$. Since $\boldsymbol{\nabla} \cdot \boldsymbol{\sigma} = \boldsymbol{\nabla} \cdot \hat{\boldsymbol{\sigma}} = \boldsymbol{0}$, we get

$$\boldsymbol{\nabla} \cdot (\boldsymbol{\sigma} \cdot \hat{\boldsymbol{u}}) - \boldsymbol{\nabla} \cdot (\hat{\boldsymbol{\sigma}} \cdot \boldsymbol{u}) = \boldsymbol{\sigma} : \boldsymbol{\nabla}\hat{\boldsymbol{u}} - \hat{\boldsymbol{\sigma}} : \boldsymbol{\nabla}\boldsymbol{u} = 2[\eta(\boldsymbol{r}) - \eta_0]\boldsymbol{E} : \boldsymbol{\nabla}\hat{\boldsymbol{u}}, \tag{S3}$$

where $\boldsymbol{E} = [\boldsymbol{\nabla}\boldsymbol{u} + (\boldsymbol{\nabla}\boldsymbol{u})^T]/2$ is the strain rate tensor corresponding to the velocity $\boldsymbol{u}$ and we use $p\boldsymbol{1} : \boldsymbol{\nabla}\hat{\boldsymbol{u}} = p(\boldsymbol{\nabla} \cdot \hat{\boldsymbol{u}}) = 0$ due to the incompressibility. Next, we integrate this identity over the fluid volume $\mathcal{V}$, and using the divergence theorem, the identity Eq. (S3) becomes

$$-\int_{\mathcal{S}} \boldsymbol{n} \cdot \boldsymbol{\sigma} \cdot \hat{\boldsymbol{u}} \, dS + \int_{\mathcal{S}} \boldsymbol{n} \cdot \hat{\boldsymbol{\sigma}} \cdot \boldsymbol{u} \, dS = 2\int_{\mathcal{V}} [\eta(\boldsymbol{r}) - \eta_0]\boldsymbol{E} : \boldsymbol{\nabla}\hat{\boldsymbol{u}} \, dV, \tag{S4}$$

where $\mathcal{S}$ is the surface of the microswimmer and $\boldsymbol{n}$ is the normal surface vector directed into the fluid. This integral theorem describes the behavior of Stokes fluids with viscosity gradients.

## S2. SWIMMING SPEEDS OF CHIRAL SQUIRMERS IN VISCOSITY GRADIENTS

We solve the swimming problem using a regular perturbation expansion of $\varepsilon$ in Eq.(5) in the main text. Applying this perturbation expansion of $\varepsilon$ to Eq. (S4), we obtain

$$-\int_{\mathcal{S}} \boldsymbol{n} \cdot \boldsymbol{\sigma} \cdot \hat{\boldsymbol{u}} \, dS + \int_{\mathcal{S}} \boldsymbol{n} \cdot \hat{\boldsymbol{\sigma}} \cdot \boldsymbol{u} \, dS = 2\varepsilon \int_{\mathcal{V}} \eta_1 \boldsymbol{E}_0 : \boldsymbol{\nabla}\hat{\boldsymbol{u}} \, dV, \tag{S5}$$

where $\boldsymbol{E}_0$ is the strain-rate tensor corresponding to the zeroth-order (Stokes limit) velocity $\boldsymbol{u}_0$. To derive the swimming speeds of chiral squirmers, we use Eq. (S5) and consider the auxiliary problem of a no-slip passive particle, denoted with the hat $\hat{}$. The boundary conditions for both active and passive particles are

$$\boldsymbol{u}|_{r=a} = \boldsymbol{U} + a\boldsymbol{\Omega} \times \boldsymbol{n} + \boldsymbol{u}^{\mathcal{S}}, \tag{S6a}$$
$$\hat{\boldsymbol{u}}|_{r=a} = \hat{\boldsymbol{U}} + a\hat{\boldsymbol{\Omega}} \times \boldsymbol{n}. \tag{S6b}$$

In uniform Stokes fluids, the flow around a translating and rotating no-slip particle is a superposition of a Stokeslet and a source dipole and a rotlet, respectively [S3],

$$\hat{\boldsymbol{u}} = \hat{\boldsymbol{u}}^U + \hat{\boldsymbol{u}}^\Omega, \tag{S7a}$$
$$\hat{\boldsymbol{u}}^U = \hat{\boldsymbol{L}}^U \cdot \hat{\boldsymbol{U}} = \left[\frac{3}{4}a\left(\frac{\boldsymbol{1}}{r} + \frac{\boldsymbol{nn}}{r}\right) + \frac{1}{4}a^3\left(\frac{\boldsymbol{1}}{r^3} - \frac{3\boldsymbol{nn}}{r^3}\right)\right] \cdot \hat{\boldsymbol{U}}, \tag{S7b}$$
$$\hat{\boldsymbol{u}}^\Omega = \hat{\boldsymbol{L}}^\Omega \cdot \hat{\boldsymbol{\Omega}} = \left(\frac{a}{r}\right)^3 \hat{\boldsymbol{\Omega}} \times \boldsymbol{r}. \tag{S7c}$$

The corresponding surface traction $\hat{\boldsymbol{f}} = \boldsymbol{n}\cdot\hat{\boldsymbol{\sigma}}|_{r=a}$, as well as the force $\hat{\boldsymbol{F}}$ and torque $\hat{\boldsymbol{T}}$ acting on the particle are given by,

$$\hat{\boldsymbol{f}} = \hat{\boldsymbol{f}}^U + \hat{\boldsymbol{f}}^\Omega, \tag{S8a}$$

$$\hat{\boldsymbol{f}}^U = -\frac{3\eta_0}{2a}\hat{\boldsymbol{U}}, \qquad \hat{\boldsymbol{f}}^\Omega = -3\eta_0\hat{\boldsymbol{\Omega}}\times\boldsymbol{n}, \tag{S8b}$$

$$\hat{\boldsymbol{F}} = \int_{\mathcal{S}} \hat{\boldsymbol{f}}\; dS = -6\pi\eta_0 a\hat{\boldsymbol{U}}, \qquad \hat{\boldsymbol{T}} = \int_{\mathcal{S}} \boldsymbol{r}\times\hat{\boldsymbol{f}}\; dS = -8\pi\eta_0 a^3\hat{\boldsymbol{\Omega}}. \tag{S8c}$$

Using Eqs. (S5)-(S8) and considering that squirmers move under force-free and torque-free conditions, we derive the swimming velocities,

$$\boldsymbol{U} = -\frac{1}{4\pi a^2}\int_{\mathcal{S}} \boldsymbol{u}^{\mathcal{S}}\; dS - \frac{\varepsilon}{3\pi\eta_0 a}\int_{\mathcal{V}} \eta_1 \boldsymbol{E}_0 : \boldsymbol{\nabla}\hat{\boldsymbol{L}}^U\; dV, \tag{S9a}$$

$$\boldsymbol{\Omega} = -\frac{3}{8\pi a^3}\int_{\mathcal{S}} \boldsymbol{n}\times\boldsymbol{u}^{\mathcal{S}}\; dS - \frac{\varepsilon}{4\pi\eta_0 a^3}\int_{\mathcal{V}} \eta_1 \boldsymbol{E}_0 : \boldsymbol{\nabla}\hat{\boldsymbol{L}}^\Omega\; dV. \tag{S9b}$$

The first terms of translational and angular velocities correspond to the swimming speed of a squirmer in the Stokes limit (the zeroth-order solution). The zeroth-order swimming velocities are $\boldsymbol{U}_0 = \boldsymbol{U}_N = (2/3)B_1\mathbf{p}$ and $\boldsymbol{\Omega}_0 = \mathbf{0}$ with the swimming axis $\mathbf{p}$. The zeroth-order solution for $\boldsymbol{u}_0$ is given as [S4],

$$\boldsymbol{u}_0 = \frac{2}{3}B_1\frac{a^3}{r^3}\mathbf{p} + B_1\frac{a^3}{r^3}\sin\theta\boldsymbol{e}_\theta + \frac{3}{2}C_2\frac{a^3}{r^3}\sin 2\theta\boldsymbol{e}_\phi. \tag{S10}$$

We compute the translational and angular velocities $(\boldsymbol{U},\boldsymbol{\Omega})$ for chiral squirmers in linear viscosity fields up to $\mathcal{O}(\varepsilon)$,

$$\boldsymbol{U} = \boldsymbol{U}_0 = \frac{2}{3}B_1\mathbf{p}, \tag{S11a}$$

$$\begin{aligned}\boldsymbol{\Omega} &= -\frac{B_1}{3}\mathbf{p}\times\boldsymbol{\nabla}\left(\frac{\eta}{\eta_0}\right) + \frac{2}{5}C_2(\mathbf{1}-3\mathbf{dd})\cdot\boldsymbol{\nabla}\left(\frac{\eta}{\eta_0}\right)\\ &= \Omega_{\mathrm{Sp}}(\boldsymbol{e}_\eta\cdot\mathbf{d})\mathbf{d} + \Omega_{\mathrm{Pr}}\boldsymbol{e}_\eta + \Omega_{\mathrm{Da}}\boldsymbol{e}_\eta\times\mathbf{p}.\end{aligned} \tag{S11b}$$

## S3. ORIENTATION DYNAMICS IN THE BODY FRAME

We describe the rotation of the chiral squirmer with $\mathbf{d}\neq\mathbf{p}$ using the Euler angles $(\varphi,\vartheta,\psi)$. The rotation follows the $zxz$-convention, which is composed of a rotation of angle $\varphi$ about $\boldsymbol{e}_z = \boldsymbol{e}_\eta$, a rotation of $\vartheta$ about the $x$ axis of the new frame, and finally a rotation of $\psi$ around the body-fixed axis $\boldsymbol{e}_3 = \mathbf{p}$. The rotation matrix $\mathbf{R}$ that transforms the laboratory frame basis vectors to the body-fixed basis vectors is given by,

$$\mathbf{R} = \begin{pmatrix} \cos\varphi\cos\psi - \sin\varphi\cos\vartheta\sin\psi & \sin\varphi\cos\psi + \cos\varphi\cos\vartheta\sin\psi & \sin\vartheta\sin\psi \\ -\cos\varphi\sin\psi - \sin\varphi\cos\vartheta\cos\psi & -\sin\varphi\sin\psi + \cos\varphi\cos\vartheta\cos\psi & \sin\vartheta\cos\psi \\ \sin\varphi\sin\vartheta & -\cos\varphi\sin\vartheta & \cos\vartheta \end{pmatrix} \tag{S12}$$

The inverse transformation is given by

$$(\boldsymbol{e}_x,\boldsymbol{e}_y,\boldsymbol{e}_z) = \mathbf{R}^T\cdot(\boldsymbol{e}_1,\boldsymbol{e}_2,\boldsymbol{e}_3). \tag{S13}$$

We can express the axis of viscosity gradients as $\boldsymbol{e}_\eta = \sin\vartheta\sin\psi\boldsymbol{e}_1 + \sin\vartheta\cos\psi\boldsymbol{e}_2 + \cos\vartheta\boldsymbol{e}_3$. The angular velocity of the swimmer can be expressed in terms of the derivatives of the Euler angles as

$$\boldsymbol{\Omega} = (\dot\varphi\sin\vartheta\sin\psi + \dot\vartheta\cos\psi)\boldsymbol{e}_1 + (\dot\varphi\sin\vartheta\cos\psi - \dot\vartheta\sin\psi)\boldsymbol{e}_2 + (\dot\varphi\cos\vartheta + \dot\psi)\boldsymbol{e}_3. \tag{S14}$$

By representing $\mathbf{d} = \sin\gamma\boldsymbol{e}_1 + \cos\gamma\boldsymbol{e}_3$ without loss of generality, and substituting into Eq. (S11b), we obtain

$$\begin{aligned}\boldsymbol{\Omega} =& \Omega_{\mathrm{Sp}}(\sin\gamma\sin\vartheta\sin\psi + \cos\gamma\cos\vartheta)(\sin\gamma\boldsymbol{e}_1 + \cos\gamma\boldsymbol{e}_3) + \Omega_{\mathrm{Pr}}(\sin\vartheta\sin\psi\boldsymbol{e}_1 + \sin\vartheta\cos\psi\boldsymbol{e}_2 + \cos\vartheta\boldsymbol{e}_3)\\ &+ \Omega_{\mathrm{Da}}(\sin\vartheta\cos\psi\boldsymbol{e}_1 - \sin\vartheta\sin\psi\boldsymbol{e}_2).\end{aligned} \tag{S15}$$

Equating the two expressions for the angular velocity (Eqs. (S14) and (S15)), we obtain the following equation [Eq.(13) in the main text],

$$\dot{\varphi} = \Omega_{\mathrm{Sp}} \left( \sin^2 \gamma \sin^2 \psi + \frac{\sin \gamma \cos \gamma \sin \psi}{\tan \vartheta} \right) + \Omega_{\mathrm{Pr}}, \tag{S16a}$$

$$\dot{\vartheta} = \Omega_{\mathrm{Sp}} (\sin^2 \gamma \sin \vartheta \sin \psi \cos \psi + \sin \gamma \cos \gamma \cos \vartheta \cos \psi) + \Omega_{\mathrm{Da}} \sin \vartheta, \tag{S16b}$$

$$\dot{\psi} = \Omega_{\mathrm{Sp}} \left( \cos^2 \gamma \cos \vartheta - \sin^2 \gamma \cos \vartheta \sin^2 \psi + \sin \gamma \cos \gamma \frac{\sin^2 \vartheta - \cos^2 \vartheta}{\sin \vartheta} \sin \psi \right). \tag{S16c}$$


[S1] N. Oppenheimer, S. Navardi, and H. A. Stone, Motion of a hot particle in viscous fluids, Phys. Rev. Fluids **1**, 014001 (2016).

[S2] K. Shoele and P. S. Eastham, Effects of nonuniform viscosity on ciliary locomotion, Phys. Rev. Fluids **3**, 043101 (2018).

[S3] J. Happel and H. Brenner, *Low Reynolds number hydrodynamics: with special applications to particulate media*, Mechanics of Fluids and Transport Processes (Springer, Dordrecht, Netherlands, 1983).

[S4] O. S. Pak and E. Lauga, Generalized squirming motion of a sphere, J. Eng. Math. **88**, 1 (2014).
